# Supplementary material for: Impact of magnetic moment and anisotropy of Co$_\textrm{1-x}$Fe$_\textrm{x}$ thin films on the magnetic proximity effect of Pt
Source: arXiv:1807.09032 ancillary file (2018-07-25)
Supplement: Supplementary file 1 [file Supplemental_Material.pdf]

# - Supplemental Material -

# Impact of magnetic moment and anisotropy of $Co_{1-x}Fe_x$ thin films on the magnetic proximity effect of Pt

Panagiota Bougiatioti[1], Orestis Manos[1], Olga Kuschel[2], Joachim Wollschläger[2], Martin Tolkiehn[3], Sonia Francoual[3], and Timo Kuschel[1]
[1] *Center for Spinelectronic Materials and Devices, Department of Physics, Bielefeld University, Universitätsstraße 25, 33615 Bielefeld, Germany*
[2] *Department of Physics and Center of Physics and Chemistry of New Materials, Osnabrück University, Barbarastraße 7, 49076 Osnabrück, Germany*
[3] *Deutsches Elektronen-Synchrotron DESY, Notkestraße 85, 22607 Hamburg, Germany*

(Dated: July 23, 2018)

## I. THEORETICAL AND EXPERIMENTAL BACKGROUND FOR XRMR

A fundamental theoretical background behind XRMR is obtained while considering the refractive index of the material under investigation exposed in x-rays, which is given by $n = 1 - \delta + i\beta$. The parameters $\delta$ and $\beta$ are the dispersion and absorption coefficients, respectively, which are connected via the Kramers-Kronig relation. When the magnetization reaches the saturation state (here H=±80 mT), the optical parameters $\delta$ and $\beta$ vary by a fraction $\pm\Delta\delta$ and $\pm\Delta\beta$, respectively, due to the magnetic circular dichroism in the material. These magnetooptic parameters are most pronounced at energies around the absorption edge of the material and vanish far from the resonance.

A six-circle diffractometer at the DESY beamline P09 was used to perform x-ray reflectivity (XRR) scans in a $\theta - 2\theta$ scattering geometry, at RT. XRR scans were collected using circularly polarized x-rays while reversing their helicity. The external magnetic field of ±80 mT was applied with a four coils electromagnet during the reflectivity scan. The XRMR data were collected at a fixed energy close to the peak of the Pt $L_3$ absorption edge (11565 eV). The degree of circular polarization was (99±1)% for left and right circularly polarized light, as determined from a polarization analysis with a Au(111) analyzer crystal. The circular polarization was achieved by one single quarter-wave-plate of 850 $\mu$m thickness.

The evaluation of the XRR data and the XRMR asymmetry ratios were performed using the analysis tool ReMagX [1]. The fitting algorithm for the nonmagnetic reflectivity data was based on the recursive Parratt algorithm, the roughness was modeled within a Névot-Croce approximation, and for the asymmetry ratio the fitting routine was based on the Zak matrix formalism, as mentioned in previous publications [2, 3]. Additional information about the XRMR technique is provided in Refs. [2–5].

Using the *ab initio* calculations for the $L_3$ absorption edge of a spin-polarized Pt thin film as reported in Ref. [2], we aligned the theoretical spectrum with the experimentally obtained XAS spectrum across the edge, for all samples. Thus, the simulated spectrum was shifted by 0.23 eV to higher energies to fit the experimental data. In turn, the dependence of the magnetooptic parameters $\Delta\delta$ and $\Delta\beta$ on the photon energy can be extracted from the simulation of the Pt absorption edge. The variation of the dispersion $\Delta\delta$ crossed zero around the absorption edge and for that reason we kept $\Delta\delta = 0$ during the XRMR fits. The change in absorption $\Delta\beta$ was positive and presented a maximum slightly shifted to lower energies with respect to the whiteline of the absorption spectrum. This is in agreement with previous publications [2–4, 6], reporting that the maximum of the magnetic dichroism for Pt is located slightly below the absorption edge. Therefore, in this photon energy range the XRMR asymmetry ratio is expected to be most evident. Finally, by comparing the resulting $\Delta\beta$ values to the *ab initio* calculations [2], the magnetic moment per spin polarized Pt atom was identified.

## II. EXTRACTED Pt MAGNETIC MOMENTS

The magnetic moments per spin polarized Pt atom for all samples as extracted from the maximum of the magnetooptic profiles in the XRMR measurements, are presented in Table I. For completeness, the magnetic moment of the Pt/Fe sample is taken from Ref. [2], where a similar sample with comparable thicknesses was used. A pronounced

TABLE I. Induced Pt magnetic moment in Pt/$Co_{1\text{-}x}Fe_x$ bilayers extracted from XRMR measurements. [1]Value taken from Ref. [2].

| Composition | Magnetic moment $\mu_B$/spin polarized Pt atom |
|---|---|
| Pt/Fe[1] | $0.60 \pm 0.10$ |
| Pt/$Co_{33}Fe_{67}$ | $0.72 \pm 0.03$ |
| Pt/$Co_{50}Fe_{50}$ | $0.71 \pm 0.03$ |
| Pt/$Co_{70}Fe_{30}$ | $0.66 \pm 0.03$ |
| Pt/$Co_{85}Fe_{15}$ | $0.49 \pm 0.03$ |
| Pt/Co | $0.43 \pm 0.03$ |

behaviour is clearly displayed with increasing Pt moment for higher Fe content values, peaking at the Pt/$Co_{33}Fe_{67}$ bilayer.


[1] S. Macke and E. Goering, J. Phys.: Condens. Matter **26**, 363201 (2014).

[2] T. Kuschel, C. Klewe, J.-M. Schmalhorst, F. Bertram, O. Kuschel, T. Schemme, J. Wollschläger, S. Francoual, J. Strempfer, A. Gupta, M. Meinert, G. Götz, D. Meier, and G. Reiss, Phys. Rev. Lett. **115**, 097401 (2015).

[3] C. Klewe, T. Kuschel, J.-M. Schmalhorst, F. Bertram, O. Kuschel, J. Wollschläger, J. Strempfer, M. Meinert, and G. Reiss, Phys. Rev. B **93**, 214440 (2016).

[4] T. Kuschel, C. Klewe, P. Bougiatioti, O. Kuschel, J. Wollschläger, L. Bouchenoire, S. D. Brown, J. M. Schmalhorst, D. Meier, and G. Reiss, IEEE Trans. Magn. **52**, 4500104 (2016).

[5] P. Bougiatioti, C. Klewe, D. Meier, O. Manos, O. Kuschel, J. Wollschläger, L. Bouchenoire, S. D. Brown, J.-M. Schmalhorst, G. Reiss, and T. Kuschel, Phys. Rev. Lett. **119**, 227205 (2017).

[6] J. Geissler, E. Goering, M. Justen, F. Weigand, G. Schütz, J. Langer, D. Schmitz, H. Maletta, and R. Mattheis, Phys. Rev. B **65**, 020405 (2001).
